# Supplementary material for: LeGo-Drive: Language-enhanced Goal-oriented Closed-Loop End-to-End Autonomous Driving
Source: arXiv:2403.20116 source file (2024-03-29)
Supplement: Supplementary file 1 [file 07_appendix.tex]

\section{Appendix}\label{appendix}

\subsection{Frenet Frame and Trajectory Parametrization}

\noindent We assume access to a lane center-line which allows us to perform motion planning in the so-called Frenet frame. In this set-up, the $X$ and $Y$ axes of the Frenet-frame are aligned with the longitudinal and lateral motion of the ego-vehicle. We parametrize the positional space ($x(k), y(k)$) of the ego-vehicle  in the Frenet frame at any time instant $k$ in terms of polynomials:

\vspace{-0.3cm}

\small
\begin{align}
    \begin{bmatrix}
        x[0],x[1], \dots, x[k] 
    \end{bmatrix} = \textbf{W}\textbf{c}_{x},
     \begin{bmatrix}
        y[0], y[1], \dots, y[k] 
    \end{bmatrix} = \textbf{W}\textbf{c}_{y},
    \label{param}
\end{align}
\normalsize

\noindent where, $\textbf{W}$ is a matrix formed with time-dependent polynomial basis functions and ($\textbf{c}_{x}, \textbf{c}_{y}$) are the coefficients of the polynomial. We can also express the derivatives in terms of $\dot{\textbf{W}}, \ddot{\textbf{W}}$. 

\subsection{Trajectory Sampling Via Setpoints}

\noindent Instead of trajectories, we follow the intuition of \cite{hoel_rl_behavior}, \cite{shrestha2023end} and sample set-points for forward velocity and lateral-offset from the center-line. These are converted to a trajectory distribution by solving the following optimization problem. 

\small
\begin{subequations}
\begin{align}
  \min  \sum_k c_{s} +c_{l}+c_v\label{cost} \\
    (x^{(r)}[0],  y^{(r)}[0]) = \textbf{b}_0 \label{boundary_cond}
\end{align}
\end{subequations}
\normalsize
\vspace{-0.5cm}
\small
\begin{subequations}
\begin{align}
    c_{s} (\ddot{x}[k], \ddot{y}[k]) = \ddot{x}[k]^2+\ddot{y}[k]^2\\
    c_{l}(\ddot{y}[k], \dot{y}[k]) = (\ddot{y}[k]-\kappa_p(y([k]y_d)-\kappa_v\dot{y}[k])^2\\
    c_v(\dot{x}[k], \ddot{x}[k]) = (\ddot{x}[k]-\kappa_p(\dot{x}[k]-v_d))^2
\end{align}
\end{subequations}
\normalsize

\noindent The first term $c_s(.)$ in the cost function \eqref{cost} ensures smoothness in the planned trajectory by penalizing high accelerations at discrete time instants. The last two terms ($c_l(.), c_v(.)$) model the tracking of lateral offset ($y_{d}$) and forward velocity $(v_{d})$ set-points respectively and is inspired from works like \cite{hoel_rl_behavior}. For the former, we define a Proportional Derivative (PD) like tracking with gain $(\kappa_p, \kappa_v)$. It induces lateral accelerations that will make the ego-vehicle converge to the $y_d$. The derivative terms in $c_l$ minimize oscillations while converging to the desired lateral offset. For velocity tracking, we only use a proportional term.  Equality constraints \eqref{boundary_cond} ensures boundary conditions on  the $r^{th}$ derivative of the planned trajectory. We use $r= \{0, 1, 2\}$ in our formulation.

Optimization \eqref{cost}-\eqref{boundary_cond} can be converted into the following QP using the trajectory parameterization of \eqref{param}.

\small
\begin{subequations}
\begin{align}
    \boldsymbol{\xi}^* = \argmin_{\boldsymbol{\xi}} \frac{1}{2}\boldsymbol{\xi}^T\textbf{Q}\boldsymbol{\xi}+\textbf{q}^T(\textbf{p})\boldsymbol{\xi}, \label{lower_cost_reform}  \\
    \textbf{A}\boldsymbol{\xi} = \textbf{b}\label{lower_eq_reform} 
    % \textbf{g}(\boldsymbol{\xi}) \leq  \textbf{0}, \label{lower_ineq}
\end{align}
\end{subequations}
\normalsize
\noindent where $\boldsymbol{\xi} = (\textbf{c}_x, \textbf{c}_y)$ and $\textbf{p} = (v_d, y_d)$. 

\begin{table*}[!t]
\centering
\caption{\scriptsize{List of Inequality Constraints Used in the projection optimization}}
\small 
\begin{tabular}{|c|c|c|c|c|c|}
\hline
Constraint Type & Expression & Parameters   \\ \hline
Collision Avoidance  & $-\frac{(x(t)-x_{o, i}(t))^2}{a^2}-\frac{(y(t)-y_{o, i}(t))^2}{b^2}+1\leq 0$ & \makecell{$\frac{a}{2}, \frac{b}{2}$: axis of the circumscribing ellipse \\ of vehicle footprint. \\ $x_{o,i}(t), y_{o, i}(t)$: trajectory of neighboring vehicles} \\ \hline
Velocity bounds & $\sqrt{\dot{x}(t)^2+\dot{y}(t)^2}\leq v_{max}$ & $v_{max}$: maximum velocity of the ego-vehicle   \\ \hline
Acceleration bounds & $\sqrt{\ddot{x}(t)^2+\ddot{y}(t)^2}\leq a_{max}$ & $a_{max}$: maximum acceleration of the ego-vehicle  \\ \hline
Lane boundary & $l_{lb}\leq y(t)\leq l_{ub}$ & \makecell{$y_{lb}, y_{ub}$: Lane bounds.} \\ \hline
\end{tabular}
\normalsize
\label{ineq_list}
\vspace{-0.6cm}
\end{table*}
\normalsize

Our trajectory planner consists of QP \eqref{lower_cost_reform}-\eqref{lower_eq_reform} augmented with a differentiable projection module. Second, the behavioural inputs are sampled from a learned distribution. We present the first component next.

\subsection{Differentiable Constrained Optimizer}

\noindent Our projection optimizer is based on \cite{shrestha2023end}
\small
\begin{align}
    \overline{\boldsymbol{{\xi}}}^{*}_j = \arg\min_{\overline{\boldsymbol{\xi}}^*_j} \frac{1}{2}\Vert \overline{\boldsymbol{\xi}}^*_j-\boldsymbol{\xi}^*_j\Vert_2^2 \label{projection_cost}\\
    \textbf{A}\overline{\boldsymbol{\xi}}^*_j = \textbf{b}(\textbf{p}_j), \qquad \textbf{g}(\overline{\boldsymbol{\xi}}^*_j) \leq  \textbf{0} \label{projection_const}
\end{align}
\normalsize

\noindent The cost function \eqref{projection_cost} aims to perform a minimal change to the output of the QP \eqref{lower_cost_reform}-\eqref{lower_eq_reform} in order to satisfy the constraints. The inequalities in \eqref{projection_const} model collision avoidance, kinematic and lane bounds. We present their algebraic form in Appendix \ref{appendix}. Therein, we also show that inequality constraints can be reformulated to induce a special structure in our projection optimization. In particular, \eqref{projection_cost}-\eqref{projection_const} can be reduced to the fixed point iterations \eqref{fixed_point_1}-\eqref{fixed_point_2}, wherein $k$ represents the iteration index.

\small
\begin{align}
    {^{k+1}}\textbf{e}_j, {^{k+1}}\boldsymbol{\lambda}_j = \textbf{h} ({^k} \overline{\boldsymbol{\xi}}_j^*, {^k}\boldsymbol{\lambda}_j ) \label{fixed_point_1}\\
    {^{k+1}}\overline{\boldsymbol{\xi}}^*_j = \arg\min_{\overline{\boldsymbol{\xi}}^*_j} \frac{1}{2}\Vert \overline{\boldsymbol{\xi}}^*_j-\boldsymbol{\xi}^*_j\Vert_2^2 +\frac{\rho}{2} \left\Vert \textbf{F}\overline{\boldsymbol{\xi}}_j^* -{^{k+1}}\textbf{e}_{j} \right\Vert_2^2\nonumber \\-{^{k+1}}\boldsymbol{\lambda}_j^T\overline{\boldsymbol{\xi}}_j^*, \qquad \textbf{A}\overline{\boldsymbol{\xi}}^*_j = \textbf{b}(\textbf{p}_j) \label{fixed_point_2}
\end{align}
\normalsize

\noindent In \eqref{fixed_point_1}-\eqref{fixed_point_2},  $\textbf{F}$ represents a constant matrix and $\textbf{h}$ is some closed-form analytical function. 
We derive these entities in  Appendix \ref{appendix}. The main cost of projection optimization stems from solving the QP \eqref{fixed_point_2}. However, since there are no inequality constraints in \eqref{fixed_point_2}, the QP essentially boils down to an affine transformation of the following form:

\small
\begin{align}
    ({^{k+1}}\overline{\boldsymbol{\xi}}^*_j, {^{k+1}}\nu) = \textbf{M}\boldsymbol{\eta}({^k} \overline{\boldsymbol{\xi}}_j^*),
    \label{affine_trans}
\end{align}
\begin{align}
    \textbf{M} = \begin{bmatrix}
        \textbf{I}+\rho\textbf{F}^T\textbf{F} & \textbf{A}^{T} \\ 
        \textbf{A} & \textbf{0}
    \end{bmatrix}^{-1}, \boldsymbol{\eta} = \begin{bmatrix}
        -\rho\textbf{F}^T {^{k+1}}\textbf{e}_j+{^{k+1}}\boldsymbol{\lambda}_j+\boldsymbol{\xi}_j^*\\
        \textbf{b}(\textbf{p}_j)
    \end{bmatrix} 
\end{align}
\normalsize

The following important features of our projection optimizer are crucial for building our end-to-end learning pipeline \cite{shrestha2023end}.

\noindent \textbf{Differentiability:} Both the $\textbf{h}(.)$ and $QP(.)$ blocks are differentiable since the former is a closed-form function and the latter reduces to simply an affine transformation \eqref{affine_trans}. 

\noindent \textbf{Batchable Structure:} Besides, being differentiable, we need the projection optimizer to be batchable for it to be easily embedded into the neural network pipeline \cite{amos2017optnet}. In other words, we should be able to compute the projection for several $\boldsymbol{\xi}_j^*$ in parallel.

% \subsection{Reformulating Constraints:} 
\noindent \textbf{Reformulating Constraints:} Table \ref{ineq_list} presents the list of all the constraints included in our projection optimizer. The collision avoidance constraints presented there can be re-written in the following form:

\small
\begin{align}
    \textbf{f}_{o, i} = \left \{ \begin{array}{lcr}
x(t) -x_{o, i}(t)-d_{o, i}(t)\cos\alpha_{o, i}(t) \\
y(t) -y_{o, i}(t)-d_{o, i}(t)\sin\alpha_{o, i}(t) \\ 
\end{array} \right \} d_{o, i}(t)\geq 1
\label{sphere_proposed}
\end{align}
\normalsize
\vspace{-0.1cm}
\noindent where $\alpha_{o, i}(t)$ represents the angle that the line-of-sight vector between the ego-vehicle and its $i^{th}$ neighbor makes with the $X$ axis. Similarly, the variable $d_{o, i}(t)$ represents the ratio of the length of this vector with the minimum distance separation required for collision avoidance. Following a similar approach, we can rephrase the velocity and acceleration bounds from Table \ref{ineq_list} as:

\vspace{-0.3cm}

\small
\begin{align}
    \textbf{f}_{v} = \left \{ \begin{array}{lcr}
\dot{x}(t) -d_{v}(t)\cos\alpha_{v}(t) \\
\dot{y}(t) -d_{v}(t)\sin\alpha_{v}(t)\\ 
\end{array} \right \}, v_{min}\leq d_{v}(t)\leq v_{max}
\label{vel_bound_proposed}
\end{align}
\normalsize

\vspace{-0.5cm}
\small
\begin{align}
    \textbf{f}_{a} = \left \{ \begin{array}{lcr}
\ddot{x}(t) -d_{a}(t)\cos\alpha_{a}(t) \\
\ddot{y}(t) -d_{a}(t)\sin\alpha_{a}(t)\\ 
\end{array} \right \}, 0\leq d_{a}(t)\leq a_{max}
\label{acc_bound_proposed}
\end{align}
\normalsize

The variables $\alpha_{o, i}(t)$, $\alpha_{o, i}(t)$, $\alpha_{a, i}(t)$, $d_{o, i}(t)$, $d_{v, i}(t)$, and $d_{a, i}(t)$  are additional variables that our batch projection optimizer will obtain along with $\overline{\boldsymbol{\xi}}_j^*$.

% \subsubsection{Reformulated Problem} 
\noindent \textbf{Reformulated Problem:} Using the developments in the previous section and the trajectory parametrization presented in \eqref{param}, we can now replace the projection optimization \eqref{projection_cost}-\eqref{projection_const} with the following. Note that \eqref{lane_reform} is the matrix representation of the lane boundary constraints presented in Table \ref{ineq_list}.

\vspace{-0.8cm}
\small
\begin{subequations}
\begin{align}
    \overline{\boldsymbol{\xi}}_j^{*} = \arg\min_{\overline{\boldsymbol{\xi}}^*_j}\frac{1}{2}\Vert \overline{\boldsymbol{\xi}}^*_j-{\boldsymbol{\xi}}_j^*\Vert_2^2\label{cost_reform}  \\
    \textbf{A} \overline{\boldsymbol{\xi}}^*_j= \textbf{b}(\textbf{p}_j) \label{eq_reform} \\
    \widetilde{\textbf{F}} \hspace{0.05cm} \overline{\boldsymbol{\xi}}^*_j = \widetilde{\textbf{e}}(\boldsymbol{\alpha}_j, \textbf{d}_j) \label{nonconvex_reform}  \\
    \textbf{d}_{min} \leq \textbf{d}_j\leq \textbf{d}_{max} \label{d_reform_1}\\
     \textbf{G}\overline{\boldsymbol{\xi}}^*_j \leq \textbf{y}_{lane} \label{lane_reform}
\end{align}
\end{subequations}
\normalsize
\vspace{-0.5cm}
\small
\begin{align}
    \widetilde{\textbf{F}} = \begin{bmatrix}
    \begin{bmatrix}
    \textbf{F}_{o}\\
    \dot{\textbf{W}}\\
    \ddot{\textbf{W}}
    \end{bmatrix} & \textbf{0}\\
    \textbf{0} & \begin{bmatrix}
    \textbf{F}_{o}\\
    \dot{\textbf{W}}\\
    \ddot{\textbf{W}}
    \end{bmatrix} 
    \end{bmatrix}, \widetilde{\textbf{e}} = \begin{bmatrix}
    \textbf{x}_o+a \textbf{d}_{o, j}\cos\boldsymbol{\alpha}_{o, j}\\
     \textbf{d}_{v, j}\cos\boldsymbol{\alpha}_{v, j}\\
  \textbf{d}_{a, j}\cos\boldsymbol{\alpha}_{a, j}\\
 \textbf{y}_o+a \textbf{d}_{o, j}\sin\boldsymbol{\alpha}_{o, j}\\
     \textbf{d}_{v, j}\sin\boldsymbol{\alpha}_{v, j}\\
  \textbf{d}_{a, j}\sin\boldsymbol{\alpha}_{a, j}\\
    \end{bmatrix},
\end{align}
\vspace{-0.3cm}
\begin{align}
    \textbf{G} = \begin{bmatrix}
        \textbf{W}\\
        -\textbf{W}
    \end{bmatrix}, \textbf{y}_{lane} = \begin{bmatrix}
        y_{ub} & \dots y_{ub} & y_{lb} \dots y_{lb}
    \end{bmatrix}^T
\end{align}
\vspace{-0.3cm}
\begin{align*}
    \boldsymbol{\alpha}_j = (\boldsymbol{\alpha}_{o, j}, \boldsymbol{\alpha}_{a,j}, \boldsymbol{\alpha}_{v,j}), \qquad \textbf{d}_j =  (\textbf{d}_{o, j}, \textbf{d}_{v, j}, \textbf{d}_{a, j})
\end{align*}
\normalsize

\noindent Constraints \eqref{nonconvex_reform}-\eqref{lane_reform} acts as substitutes for $\textbf{g}(\overline{\boldsymbol{\xi}}_j^*)\leq 0 $ in the projection optimization \eqref{projection_cost}-\ref{projection_const}. 
% Please also note the addition of subscript $j$ indicating that the \eqref{cost_reform}-\eqref{lane_reform} is defined for the $j^{th}$ sample of ${\boldsymbol{\xi}}_j$

The matrix $\textbf{F}_o$ is obtained by stacking the matrix $\textbf{W}$ from (\ref{param}) as many times as the number of neighboring vehicles considered for collision avoidance at a given planning cycle. The vector $\textbf{x}_o, \textbf{y}_o$ is formed by appropriately stacking $x_{o, i}(t), y_{o, i}(t)$ at different time instants and for all the neighbors. Similar construction is followed to obtain $\boldsymbol{\alpha}_{o}, \boldsymbol{\alpha}_{v}, \boldsymbol{\alpha}_{a}, \textbf{d}_{o}, \boldsymbol{d}_{v}, \boldsymbol{d}_{a}$. The vector $\textbf{y}_{lane}$ is formed by stacking the upper and lower lane bounds after repeating them $m$ times (planning horizon). Similarly,  vectors $d_{min}, d_{max}$ are formed by stacking the lower and upper bounds for $d_{o, i}(t), d_a(t), d_v(t)$. Note that the upper bound for $d_{o, i}(t)$ can be simply some large number (recall \eqref{sphere_proposed}). Moreover, these bounds are the same across all batches.

% \subsubsection{Solution Process} 
\noindent \textbf{Solution Process:} We relax the non-convex equality \eqref{nonconvex_reform} and affine inequality constraints as $l_2$ penalties and augment them into the projection cost \eqref{cost_reform}.

\small
\begin{dmath}
    \mathcal{L} = \frac{1}{2}\left\Vert \overline{\boldsymbol{\xi}}^*_j-\boldsymbol{\xi}^*_j\right\Vert_2^2- \boldsymbol{\lambda}_{j}^T \overline{\boldsymbol{\xi}}^*_j+\frac{\rho}{2} \left \Vert \widetilde{\textbf{F}} \overline{\boldsymbol{\xi}}^*_j-\widetilde{\textbf{e}}\right \Vert_2^2+  \frac{\rho}{2}\left \Vert \mathbf{G} \overline{\boldsymbol{\xi}}^*_{j} - \textbf{y}_{lane} + \mathbf{s}_j \right \Vert^2 = \frac{1}{2}\left\Vert \overline{\boldsymbol{\xi}}^*_j-\boldsymbol{\xi}^*_j\right\Vert_2^2-\boldsymbol{\lambda}_{j}^T \overline{\boldsymbol{\xi}}^*_j+\frac{\rho}{2} \left \Vert \textbf{F} \overline{\boldsymbol{\xi}}^*_j-\textbf{e}\right \Vert_2^2
    \label{aug_lag}
\end{dmath}
\normalsize

\small
\begin{align}
    \textbf{F} = \begin{bmatrix}
        \widetilde{\textbf{F}}\\
        \textbf{G}
    \end{bmatrix}, \textbf{e} = \begin{bmatrix}
        \widetilde{\textbf{e}}\\
        \textbf{y}_{lane}-\textbf{s}_j
    \end{bmatrix}
\end{align}
\normalsize
\noindent Note, the introduction of the Lagrange multiplier $\boldsymbol{\lambda}$ that drives the residual of the second and third quadratic penalties to zero. We minimize \eqref{aug_lag} subject to \eqref{eq_reform} through Alternating Minimization (AM), which reduces to the following steps \cite{masnavi2022visibility}.
% \cite{split_bergman}

\vspace{-0.6cm}
\small
\begin{subequations}
    \begin{align}
        {^{k+1}\boldsymbol{\alpha}_j} = \arg\min_{\boldsymbol{\alpha}_j} \mathcal{L}({^k}\overline{\boldsymbol{\xi}}_j^*, {^k}\textbf{d}_j, \boldsymbol{\alpha}_j {^k}\boldsymbol{\lambda}_j, {^k}\textbf{s}_j ) \label{am_alpha}\\
        {^{k+1}\textbf{d}_j} = \arg\min_{\textbf{d}_j} \mathcal{L}({^k}\overline{\boldsymbol{\xi}}_j^*, \textbf{d}_j, {^{k+1}}\boldsymbol{\alpha}_j, {^k}\boldsymbol{\lambda}_j, {^k}\textbf{s}_j) \label{am_d} \\ 
        {^{k+1}}\mathbf{s}_j =\text{max}\left(0, -\mathbf{G} {^{k}}\overline{\boldsymbol{\xi}}_{j}^* - \textbf{y}_{lane}\right) \label{am_s} \\
        {^{k+1}}\boldsymbol{\lambda}_j = \overbrace{{^{k}}\boldsymbol{\lambda}_j+\rho\textbf{F}^T (\textbf{F}\hspace{0.05cm} {^k}\overline{\boldsymbol{\xi}}_j^*-{^{k}}\textbf{e}_j  )}^{\textbf{h}_1} \label{am_lambda} \\
        {^{k+1}}\textbf{e}_j = \overbrace{\begin{bmatrix}
        \widetilde{\textbf{e}} ({^{k+1}} \boldsymbol{\alpha}_j, {^{k+1}}\textbf{d}_j ) \label{am_e} \\
        \textbf{y}_{lane}-{^{k+1}}\textbf{s}_j
    \end{bmatrix}}^{\textbf{h}_2}\\
        {^{k+1}}\overline{\boldsymbol{\xi}}_j^* = \arg\min_{\overline{\boldsymbol{\xi}}_j^*}\mathcal{L}(\overline{\boldsymbol{\xi}}_j^*, {^{k+1}}\boldsymbol{\lambda}_j, {^{k+1}}\textbf{e}_j ) \label{am_xi}
    \end{align}
\end{subequations}
\normalsize

As can be seen, we optimize over only one group of variables at each AM step while others are held fixed at values obtained at the previous updates. Steps \eqref{am_lambda}-\eqref{am_e} provides the function $\textbf{h}$ presented in \eqref{fixed_point_1}. That is, $\textbf{h} = (\textbf{h}_1, \textbf{h}_2)$. Step \eqref{am_xi} represents \eqref{fixed_point_2}. An important thing to note is that \eqref{am_alpha}, \eqref{am_d} have a closed-form solution in terms of ${^{k}}\overline{\boldsymbol{\xi}}^*_j$ and thus do not require any matrix factorization \cite{masnavi2022visibility}.
